# Supplementary material for: Communicability Angle and the Spatial Efficiency of Networks
Source: arXiv:1412.7388 source file (2015-07-28)
Supplement: Supplementary file 1 [file Supplementary_Info.pdf]

# Supplementary Information

July 26, 2015

## 1 Computational methods

The communicability angles between every pair of nodes can be obtained from the communicability angles matrix, which is given by

$$An = \cos^{-1}\left\{G \oslash \left[\left(\vec{s}\cdot\vec{1}\right) \odot \left(\vec{1}\cdot\vec{s}\right)\right]\right\}^{\odot(1/2)}, \tag{1}$$

where $\oslash$ stands for the entrywise division, $\odot$ for the Hadamard product (entrywise product) of two matrices, and $\cdot$ for the inner product of two vectors. Here, $\vec{s} = diag\,(G)$, $G = \exp(A)$ and $\vec{1}$ is an all-ones vector.

In a similar way the communicability distance matrix can be obtained as

$$X = \left(\vec{s}\cdot\vec{1} + 1\vec{\cdot}\vec{s} - 2G\right). \tag{2}$$

From the computationa point of view it is clear that everything rests on the calculation of the matrix exponential. The matrix exponentail can be defined by considering the Taylor series expansion of the matrix as [1]

$$\exp(A) = I + A + \frac{A^2}{2!} + \cdots = \sum_{k=0}^{\infty}\frac{A^k}{k!}. \tag{3}$$

However, it is not recommended under any circunstances to use the Taylor series expansion to compute the matrix exponential. There are many ways of doing this computation more efficiently and the reader is directed to the classic papers of Moler and Van Loan for many examples [2, 3]. From those papers it is clear that there are three or four methods that display the best performance. Among them we selected the *scaling and squaring method*, which is implemented in Matlab® and which has become by far the most widely used method for computing $\exp(A)$. In brief, the scaling and squaring method scales the matrix $A$ by a power of 2 to reduce the norm to order 1, computes a Padé approximant to the matrix exponential, and then repeatedly squares to undo the effect of the scaling. In Matlab, it is done by using the **expm** function. For an excellent review of the method, its error and accuracy the reader is referred to the classic papers by Higham [4, 5]. The time and complexity of the calculation of matrix exponential do not only depend on the matrix size, but also on the structure of such matrices. A clearer idea of the complexity and timing for adjacency matrices of netowks can be obtained from the recent paper by Benzi and Klymko [6]. The reader should also be aware of excellent bounds existing for the individual entries of the communicability matrix. For instance, using quadrature rule methods Benzi and Bioto [7] have obtained bounds for $G_{pq}$ and $G_{pp}$. Such bound can be easily implemented in cases where the size and complexity of the network impedes the use of the scaling and squaring method for the direct computation of the matrix exponential. A Matlab code is given below for computing both the communicability angle and distance matrices.

**Algorithm 1** Matlab function for obtaining the communicability angle and distance matrices.

```
function [An, X]=communicability_geom(A, beta)

%Communicability_angle
%         Generates the matrices An and X of communicability angles
%         and distances of a network.
%         The (i,j) entry of the matrix An corresponds to the
%         communicability angle between the position vectors of the nodes
%         i and j in a hyperspherical embedding of the graph.
%
%        The entry (i,j) of the matrix X corresponds to the
%         communicability distance between the nodes i and j in the graph.
%
%   Input         A: adjacency matrix
%              beta: inverse temperature. Defaults to 1
%
%
%   Output      An: n by n symmetric hollow matrix of communicability angles.
%                X: n by n symmetric hollow matrix of communicability
%                   distances.
%
%   Reference:   Estrada, Ernesto, and Naomichi Hatano.
%                "Communicability Angle and the Spatial Efficiency
%                of Networks." arXiv preprint arXiv:1412.7388 (2014).
%
%   Example: [An, X] = communicability_angle(A,1);

if nargin <= 1
   beta = 1;
end;

% Precalculations
    A=max(A,A')-diag(diag(A));
    n=length(A);
    u=ones(n,1);

% Communicability

     G=expm(beta*A);            % Communicability matrix
     sc=diag(G);                % Vector of self-communicabilities

% Comunicability angles matrix

      An=acosd(G./((sc*u').*(u*sc')).^0.5);

% Communicability distance matrix
     CD=(sc*u'+u*sc'-2*G);             %Squared Communicability distance matrix
     X=CD.^0.5;                        %Communicability distance matrix
```

## 2 Datasets

Here we give a brief description of the networks used for the tests throughout the paper.

*Brain networks*

- Neurons: Neuronal synaptic network of the nematode *C. elegans*. Included all data except muscle cells and using all synaptic connections [8]; Cat and macaque visual cortices: the brain networks of macaque visual cortex and cat cortex, after the modifications introduced by Sporn and Kötter [17].

*Ecological networks*

- Benguela: Marine ecosystem of Benguela off the southwest coast of South Africa [29]; Bridge Brook: Pelagic species from the largest of a set of 50 New York Adirondack lake food webs [19]; Canton Creek: Primarily invertebrates and algae in a tributary, surrounded by pasture, of the Taieri River in the South Island of New Zealand [20]; Chesapeake Bay: The pelagic portion of an eastern U.S. estuary, with an emphasis on larger fishes [21]; Coachella: Wide range of highly aggregated taxa from the Coachella Valley desert in southern California [22]; El Verde: Insects, spiders, birds, reptiles and amphibians in a rainforest in Puerto Rico [23]; Grassland: all vascular plants and all insects and trophic interactions found inside stems of plants collected from 24 sites distributed within England and Wales [24]; Little Rock: Pelagic and benthic species, particularly fishes, zooplankton, macroinvertebrates, and algae of the Little Rock Lake, Wisconsin, U.S. [25]; Reef Small: Caribbean coral reef ecosystem from the Puerto Rico-Virgin Island shelf complex [26]; Scotch Broom: Trophic interactions between the herbivores, parasitoids, predators and pathogens associated with broom, Cytisus scoparius, collected in Silwood Park, Berkshire, England, UK [27]; Shelf: Marine ecosystem on the northeast US shelf [28]; Skipwith: Invertebrates in an English pond [18]; St. Marks: Mostly macroinvertebrates, fishes, and birds associated with an estuarine seagrass community, Halodule wrightii, at St. Marks Refuge in Florida [30]; St. Martin: Birds and predators and arthropod prey of Anolis lizards on the island of St. Martin, which is located in the northern Lesser Antilles [31]; Stony Stream: Primarily invertebrates and algae in a tributary, surrounded by pasture, of the Taieri River in the South Island of New Zealand in native tussock habitat [32]; Ythan_1: Mostly birds, fishes, invertebrates, and metazoan parasites in a Scottish Estuary [33] ;Ythan_2: Reduced version of Ythan1 with no parasites [34].
- Termite: The networks of three-dimensional galleries in termite nests [65]; Ant: The network of galleries created by ants [66]; Dolphins: social network of frequent association between 62 bottlenose dolphins living in the waters off New Zealand [55];

*Informational networks*

- Centrality: Citation network of papers published in the field of Network Centrality [35, 36]; GD: Citation network of papers published in the Proceedings of Graph Drawing during the period 1994-2000 [37]; ODLIS: Vocabulary network of words related by their definitions in the Online Dictionary of Library and Information Science. Two words are connected if one is used in the definition of the other [38]; Roget: Vocabulary network of words related by their definitions in Roget's Thesaurus of English. Two words are connected if one is used in the definition of the other [39]; Small World: Citation network of papers that cite S. Milgram's 1967 Psychology Today paper or use Small World in title [40].

*Biological networks*

- Protein-protein interaction networks in: *Kaposi sarcoma herpes virus* (KSHV) [41]; *P. falciparum* (malaria parasite) [42]; *human* [43]; *S. cerevisiae* (yeast) [44, 45]; *A. fulgidus* [46]; *H. pylori* [47]; *C. elegans* [48]; *E. coli* [49] and *B. subtilis* [50].
- Trans_E.coli: Direct transcriptional regulation between operons in *Escherichia coli* [51, 52]; Trans_sea_urchin: Developmental transcription network for sea urchin endomesoderm development. [51]; Trans_yeast: Direct transcriptional regulation between genes in *Saccaromyces cerevisae.* [8, 51].

*Social and economic networks*

- Corporate: American corporate elite formed by the directors of the 625 largest corporations that reported the compositions of their boards selected from the Fortune 1000 in 1999 [53]; Geom: Collaboration network of scientists

in the field of Computational Geometry [40]; Prison: Social network of inmates in prison who chose "What fellows on the tier are you closest friends with?" [54]; Drugs: Social network of injecting drug users (IDUs) that have shared a needle in the last six months [56]; Zachary: Social network of friendship between members of the Zachary karate club [57]; College: Social network among college students in a course about leadership. The students choose which three members they wanted to have in a committee [58]; ColoSpring: The risk network of persons with HIV infection during its early epidemic phase in Colorado Spring, USA, using analysis of community wide HIV/AIDS contact tracing records (sexual and injecting drugs partners) from 1985-1999 [59]; Galesburg: Friendship ties among 31 physicians [36]; High_Tech: Friendship ties among the employees in a small high-tech computer firm which sells, installs, and maintain computer systems [60, 36]; Saw Mills: Social communication network within a sawmill, where employees were asked to indicate the frequency with which they discussed work matters with each of their colleagues [61, 36]; MMM: World trade network of miscellaneous manufacture of metals (MMM) in 1994 [36].

*Protein residue networks*

- Nodes represent amino acids and two nodes are connected if the corresponding amino acids are separated at less than 7Å in the crystallographic structure deposited in the Protein Data Bank (PDB). The proteins considered were transformed to protein residue networks in [11] and the ones selected here have codes: 1lfb; 9rnt; 1aep; 1jpc; 1vls; 1klo; 2aak; 1xjo; 1amm; 1mla; 1ad2; 1nox; 1akz; 1xsm; 1ako; 1han; 1air; 1gnd; 1aa6; 1alo; 1kit.

*Urban street networks*

- Nodes represent the intersections between two streets in a city and the edges represent segments of streets between two intersections [64]. The networks represent the following cities from the ones studied in [64]: Barcelona; Rio Grande; Yuliang; Chegkan; Atlanta; Berlin; Rotterdam; Hong Kong; Mecca; Cambridge; Oxford; Ahmedabad; Milton Keynes.

*Technological and infrastructural networks*

- Electronic: Three electronic sequential logic circuits parsed from the ISCAS89 benchmark set, where nodes represent logic gates and flip-flop [8]; USAir97: Airport transportation network between airports in US in 1997 [40]; Internet: The internet at the Autonomous System (AS) level as of September 1997 and of April 1998 [62]; Power Grid: The power grid network of the Western USA [63].

*Software networks*

- Collaboration networks associated with six different open-source software systems, which include collaboration graphs for three Object Oriented systems written in C++, and call graphs for three procedural systems written in C. The class collaboration graphs are from version 4.0 of the VTK visualization library; the CVS snapshot dated 4/3/2002 of Digital Material (DM), a library for atomistic simulation of materials; and version 1.0.2 of the AbiWord word processing program. The call graphs are from version 2.4.19 of the kernel of the Linux operating system, version 3.23.32 of the MySQL relational database system, and version 1.2.7 of the XMMS multimedia system. Details of the construction and/or origin of these networks are provided in Myers [9].

# 3 Results

In Table 1 we give the values of the network parameters studied in this paper as well as a few others that can give a better idea of the kind of networks we have studied here. They include: the number of nodes $n$, the number of edges $m$, the average node degree $\langle k \rangle$, the maximum node degree $k_{max}$, the average path length $\langle l \rangle$, average Watts and Strogatz clustering coefficient $\bar{C}$, the network efficiency $E$, average resistance distance $\langle \Omega \rangle$, average communicability distance $\langle \xi \rangle$ and angle $\langle \theta \rangle$. The networks belong to the following classes: biological (1-14), urban street networks (15-27), ecological networks (28-49), social networks (50-64), software networks (65-70), technological and infrastructural networks (71-77).

**Table 1.** Values of the average communicability angles of all the real-world networks studied except the protein residue networks.

| No. | Name | $n$ | $m$ | $\langle k \rangle$ | $k_{max}$ | $\langle l \rangle$ | $\bar{C}$ | $E$ | $\langle \Omega \rangle$ | $\langle \xi \rangle$ | $\langle \theta \rangle$ |
|---|---|---|---|---|---|---|---|---|---|---|---|
| 1 | PIN_yeast | 2224 | 6609 | 5.94 | 64 | 4.38 | 0.14 | 0.25 | 1.27 | 177.09 | 38.92 |
| 2 | PIN_Ecoli | 230 | 695 | 6.04 | 36 | 3.78 | 0.22 | 0.31 | 1.66 | 147.96 | 39.76 |
| 3 | PIN_KSHV | 50 | 114 | 4.56 | 16 | 2.84 | 0.13 | 0.42 | 1.13 | 5.18 | 51.59 |
| 4 | PIN_Malaria | 229 | 604 | 5.28 | 35 | 3.38 | 0.17 | 0.33 | 0.82 | 8.65 | 55.04 |
| 5 | PIN_Human | 2783 | 6007 | 4.32 | 129 | 4.84 | 0.07 | 0.22 | 1.55 | 36.32 | 58.79 |
| 6 | Trans_urchin | 45 | 80 | 3.56 | 14 | 3.22 | 0.21 | 0.39 | 2.02 | 4.22 | 61.87 |
| 7 | PIN_Hpylori | 710 | 1396 | 3.93 | 55 | 4.15 | 0.02 | 0.26 | 1.47 | 7.13 | 67.51 |
| 8 | Trans_Ecoli | 328 | 456 | 2.78 | 72 | 4.83 | 0.11 | 0.25 | 2.54 | 5.19 | 77.44 |
| 9 | PIN_Afulgidus | 32 | 36 | 2.25 | 9 | 3.60 | 0.06 | 0.35 | 2.49 | 2.18 | 79.35 |
| 10 | PIN_Bsubtilis | 84 | 98 | 2.33 | 17 | 4.05 | 0.04 | 0.29 | 2.52 | 2.52 | 81.77 |
| 11 | Trans_yeast | 662 | 1062 | 3.21 | 71 | 5.20 | 0.05 | 0.22 | 2.06 | 7.16 | 83.33 |
| 12 | cat Cortex | 52 | 515 | 19.81 | 37 | 1.64 | 0.66 | 0.69 | 0.13 | 5792.78 | 0.22 |
| 13 | neurons | 280 | 1973 | 14.09 | 77 | 2.63 | 0.28 | 0.42 | 0.26 | 4575.37 | 1.57 |
| 14 | Macaque | 32 | 194 | 12.13 | 22 | 1.66 | 0.65 | 0.69 | 0.24 | 91.52 | 3.60 |
| 15 | Barcelona | 5575 | 16060 | 5.76 | 126 | 7.94 | 0.19 | 0.15 | 1.08 | 828.39 | 71.89 |
| 16 | Rio Grande | 855 | 2702 | 6.32 | 57 | 6.90 | 0.08 | 0.18 | 1.35 | 67.23 | 79.68 |
| 17 | Yuliang | 88 | 129 | 2.93 | 7 | 6.03 | 0.17 | 0.23 | 3.22 | 2.76 | 85.84 |
| 18 | Chegkan | 414 | 1208 | 5.84 | 18 | 8.97 | 0.16 | 0.15 | 0.99 | 7.98 | 86.07 |
| 19 | Atlanta | 3234 | 7319 | 4.53 | 65 | 7.71 | 0.15 | 0.15 | 1.64 | 12.20 | 86.47 |
| 20 | Berlin | 4495 | 12889 | 5.73 | 50 | 9.24 | 0.20 | 0.13 | 1.07 | 16.46 | 88.19 |
| 21 | Rotterdam | 1300 | 2759 | 4.24 | 28 | 9.59 | 0.14 | 0.13 | 1.62 | 4.69 | 88.60 |
| 22 | Hong Kong | 916 | 1613 | 3.52 | 23 | 12.85 | 0.13 | 0.11 | 4.33 | 3.94 | 88.91 |
| 23 | Mecca | 1464 | 2789 | 3.81 | 18 | 13.44 | 0.21 | 0.10 | 1.98 | 3.79 | 89.48 |
| 24 | Cambridge | 1509 | 2190 | 2.90 | 31 | 11.15 | 0.11 | 0.11 | 3.98 | 3.08 | 89.49 |
| 25 | Oxford | 1622 | 2825 | 3.48 | 19 | 12.97 | 0.17 | 0.10 | 3.05 | 3.43 | 89.53 |
| 26 | Ahmedabad | 4874 | 7242 | 2.97 | 21 | 13.41 | 0.16 | 0.09 | 3.60 | 3.06 | 89.86 |
| 27 | Milton Keynes | 5581 | 7261 | 2.60 | 25 | 13.19 | 0.08 | 0.09 | 4.62 | 2.73 | 89.89 |
| 28 | Ants | 74 | 97 | 2.62 | 7 | 5.57 | 0.04 | 0.24 | 2.92 | 2.50 | 85.51 |
| 29 | Termite3 | 268 | 437 | 3.26 | 12 | 7.89 | 0.12 | 0.18 | 2.37 | 3.35 | 87.16 |
| 30 | Termite2 | 260 | 280 | 2.15 | 12 | 9.11 | 0.01 | 0.15 | 5.22 | 2.30 | 88.84 |
| 31 | Termite1 | 507 | 676 | 2.67 | 10 | 8.51 | 0.04 | 0.15 | 2.95 | 2.64 | 89.00 |
| 32 | Dolphins | 62 | 159 | 5.13 | 12 | 3.36 | 0.26 | 0.38 | 0.99 | 5.98 | 65.37 |
| 33 | Shelf | 81 | 1451 | 35.83 | 69 | 1.57 | 0.59 | 0.72 | 0.07 | 61317050 | 0.00 |
| 34 | Elverde | 156 | 1439 | 18.45 | 83 | 2.30 | 0.21 | 0.50 | 0.38 | 393308.86 | 0.01 |
| 35 | Skipwith | 35 | 353 | 20.17 | 32 | 1.42 | 0.63 | 0.79 | 0.11 | 3327.87 | 0.02 |
| 36 | ReefSmall | 50 | 503 | 20.12 | 39 | 1.60 | 0.61 | 0.70 | 0.14 | 8975.44 | 0.05 |
| 37 | LittleRock | 181 | 2318 | 25.61 | 105 | 2.22 | 0.35 | 0.51 | 0.25 | 37085665 | 0.05 |
| 38 | Stony | 112 | 830 | 14.82 | 45 | 2.34 | 0.07 | 0.49 | 0.45 | 5371.98 | 0.10 |
| 39 | Coachella | 30 | 241 | 16.07 | 25 | 1.46 | 0.71 | 0.77 | 0.16 | 622.10 | 0.25 |
| 40 | Canton | 108 | 707 | 13.09 | 47 | 2.35 | 0.05 | 0.49 | 0.48 | 1103.80 | 0.46 |
| 41 | Benguela | 29 | 191 | 13.17 | 24 | 1.62 | 0.57 | 0.72 | 0.26 | 160.96 | 1.23 |
| 42 | BridgeBrook | 75 | 542 | 14.45 | 41 | 2.17 | 0.20 | 0.54 | 0.30 | 2041.51 | 2.01 |

| | | | | | | | | | | | |
|---|---|---|---|---|---|---|---|---|---|---|---|
| 43 | Ythan2 | 92 | 416 | 9.04 | 50 | 2.25 | 0.22 | 0.49 | 0.53 | 180.70 | 2.03 |
| 44 | Ythan1 | 134 | 593 | 8.85 | 65 | 2.40 | 0.23 | 0.46 | 0.57 | 251.88 | 2.16 |
| 45 | StMartins | 44 | 218 | 9.91 | 27 | 1.93 | 0.33 | 0.59 | 0.37 | 41.77 | 6.15 |
| 46 | StMarks | 48 | 218 | 9.08 | 19 | 2.09 | 0.28 | 0.55 | 0.35 | 33.30 | 8.25 |
| 47 | ScotchBroom | 154 | 366 | 4.75 | 36 | 3.39 | 0.14 | 0.33 | 1.60 | 95.26 | 30.32 |
| 48 | Chesapeake | 33 | 71 | 4.30 | 10 | 2.80 | 0.20 | 0.45 | 1.09 | 3.72 | 60.69 |
| 49 | SmallW | 233 | 994 | 8.53 | 147 | 2.37 | 0.56 | 0.45 | 0.63 | 1459.4 | 5.05 |
| 50 | ODLIS | 2898 | 16376 | 11.30 | 592 | 3.17 | 0.30 | 0.34 | 0.65 | 45714627 | 0.04 |
| 51 | Roget | 994 | 3640 | 7.32 | 28 | 4.08 | 0.15 | 0.27 | 0.64 | 14.80 | 65.74 |
| 52 | GD | 249 | 635 | 5.10 | 20 | 4.15 | 0.24 | 0.28 | 1.19 | 8.32 | 75.65 |
| 53 | Centrality | 118 | 613 | 10.39 | 66 | 2.37 | 0.37 | 0.47 | 0.56 | 1025.69 | 1.01 |
| 54 | Corporate | 1586 | 11540 | 14.55 | 65 | 3.51 | 0.50 | 0.31 | 0.27 | 2099.82 | 15.54 |
| 55 | Geom | 3621 | 9461 | 5.23 | 102 | 5.32 | 0.54 | 0.21 | 1.66 | 15960.86 | 17.22 |
| 56 | HighTech | 33 | 91 | 5.52 | 16 | 2.36 | 0.45 | 0.51 | 0.79 | 7.22 | 39.20 |
| 57 | Zachary | 34 | 78 | 4.59 | 17 | 2.41 | 0.57 | 0.49 | 0.84 | 4.60 | 45.45 |
| 58 | College | 32 | 80 | 5.00 | 13 | 2.30 | 0.33 | 0.51 | 0.58 | 3.62 | 52.10 |
| 59 | Galesburg | 31 | 67 | 4.32 | 10 | 2.53 | 0.35 | 0.47 | 0.94 | 3.60 | 59.71 |
| 60 | Drugs | 616 | 2012 | 6.53 | 58 | 5.28 | 0.55 | 0.23 | 1.84 | 245.25 | 64.02 |
| 61 | SawMill | 36 | 62 | 3.44 | 13 | 3.14 | 0.31 | 0.40 | 1.40 | 2.96 | 71.41 |
| 62 | Prison | 67 | 142 | 4.24 | 11 | 3.35 | 0.31 | 0.36 | 1.06 | 3.87 | 76.54 |
| 63 | MMM | 80 | 875 | 21.88 | 77 | 1.72 | 0.75 | 0.64 | 0.14 | 185828.3 | 0.01 |
| 64 | Colospg | 324 | 347 | 2.14 | 20 | 8.33 | 0.03 | 0.15 | 5.95 | 2.48 | 88.46 |
| 65 | Linux | 5285 | 11352 | 4.30 | 1058 | 4.66 | 0.11 | 0.24 | 1.44 | 172348.6 | 3.47 |
| 66 | MySQL | 1480 | 4190 | 5.66 | 220 | 5.47 | 0.16 | 0.23 | 1.55 | 895.51 | 45.68 |
| 67 | VTK | 771 | 1357 | 3.52 | 83 | 4.53 | 0.06 | 0.24 | 1.90 | 9.78 | 70.11 |
| 68 | Abi | 1035 | 1719 | 3.32 | 89 | 5.08 | 0.06 | 0.22 | 2.31 | 9.26 | 72.86 |
| 69 | Digital | 150 | 198 | 2.64 | 25 | 4.85 | 0.05 | 0.25 | 3.02 | 3.25 | 81.62 |
| 70 | XMMS | 971 | 1802 | 3.71 | 36 | 6.35 | 0.05 | 0.18 | 2.15 | 6.50 | 84.32 |
| 71 | USAir97 | 332 | 2126 | 12.81 | 139 | 2.74 | 0.63 | 0.41 | 0.83 | 37248593 | 0.00 |
| 72 | electronic1 | 122 | 189 | 3.10 | 10 | 4.93 | 0.06 | 0.25 | 1.77 | 2.68 | 86.18 |
| 73 | electronic2 | 252 | 399 | 3.17 | 14 | 5.81 | 0.06 | 0.20 | 1.84 | 2.77 | 87.94 |
| 74 | electronic3 | 512 | 819 | 3.20 | 22 | 6.86 | 0.05 | 0.17 | 1.92 | 2.83 | 88.89 |
| 75 | PowerGrid | 4941 | 6594 | 2.67 | 19 | 18.99 | 0.08 | 0.06 | 5.23 | 2.74 | 89.91 |
| 76 | Internet98 | 3522 | 6324 | 3.59 | 742 | 3.77 | 0.19 | 0.29 | 1.65 | 375932.59 | 0.42 |
| 77 | Internet97 | 3015 | 5156 | 3.42 | 590 | 3.76 | 0.18 | 0.29 | 1.73 | 84399.95 | 0.78 |

In Fig. (1) we illustrate the scatterplots of the communicability angle versus a few of the network parameters studied in the paper for the 77 real-world networks given in Table 1. Apart from the evident lack of correlation between the pairs of measures it is interesting to notice the fact that there are pairs of networks with the same value of a given parameter, e.g., average degree, average path length, efficiency, etc., but having very different values of the communicability angle. There is one example provided in the main text of the article but many more can be extracted from these plots. Notice the plot between the communicability distance and communicability angle is semi-log scale.

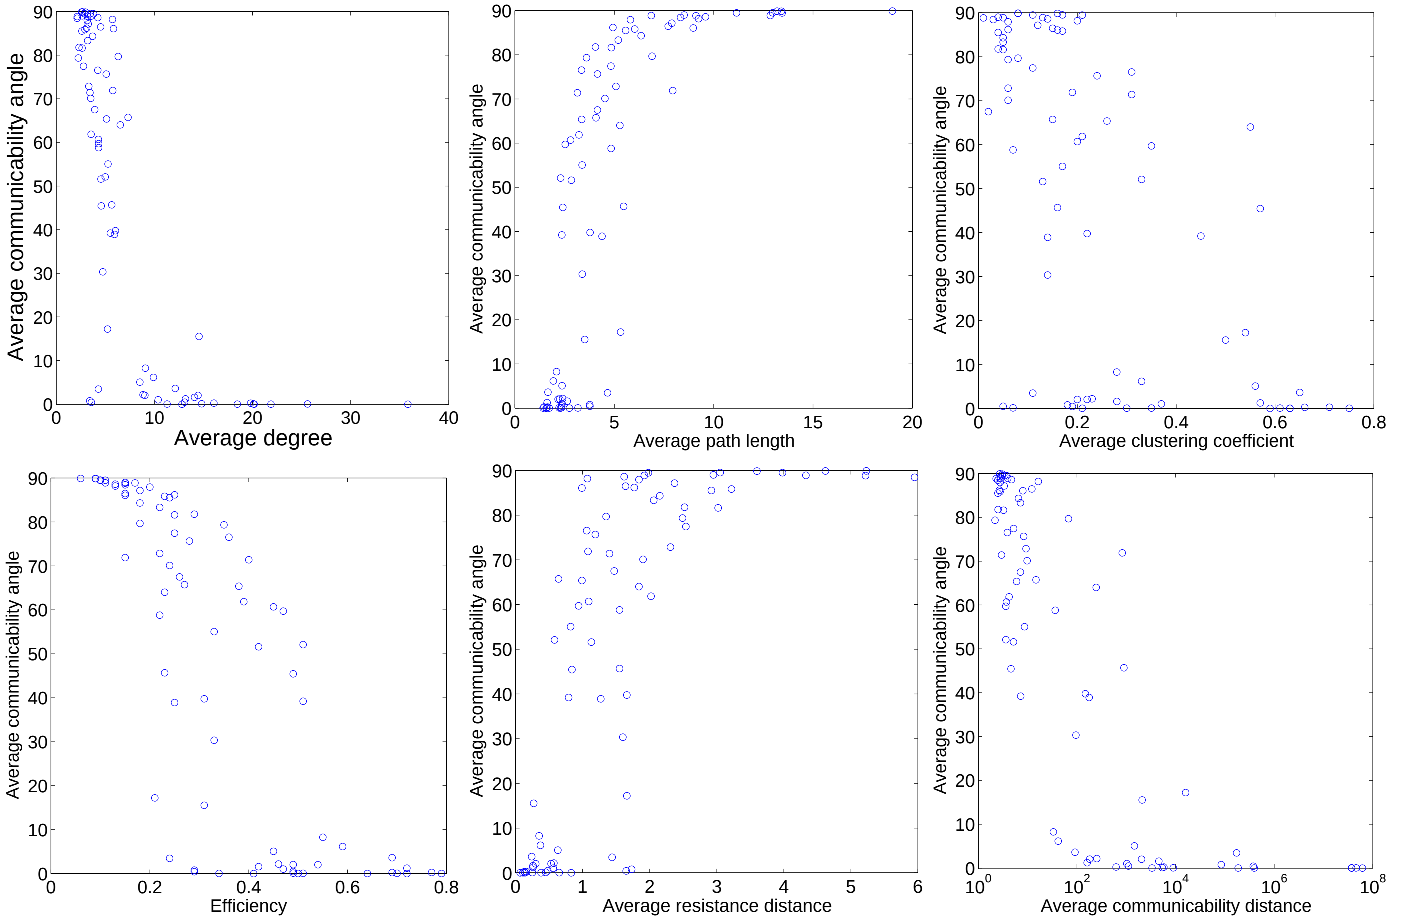


Figure 1: Scatterplots of the average communicability angle vs. a few network metrics.

**Table 2.** Values of the average communicability angles as well as the real and expected values of the volume of all the protein residue networks studied.

| PDB code | $V_o\left(\mathring{A}^3\right)$ | $V_e\left(\mathring{A}^3\right)$ | $\langle\theta\rangle$ |
|---|---|---|---|
| 1npoA | 9002.4 | 9566.2 | 64.75 |
| 1tfs | 7634.98 | 7976.8 | 65.01 |
| 1ptx | 8010.5 | 8252.9 | 65.95 |
| 1dtx | 7470.9 | 7873.5 | 68.27 |
| 5rxn | 6620.4 | 6778.5 | 68.28 |
| 1ceaA | 9869.9 | 10508 | 68.35 |
| 2abd | 10670.11 | 11518.2 | 69.69 |
| 1cdr | 10144.64 | 10349.8 | 71.09 |
| 1lfb | 10127.9 | 10658.1 | 71.78 |
| 9rnt | 12314.6 | 12960.6 | 73.93 |
| 2madL | 14881.6 | 15848.1 | 74.90 |
| 2azaA | 16295.7 | 16507 | 74.97 |
| 1fkj | 13754.5 | 13857.3 | 75.31 |
| 1rtp1 | 14006.2 | 13826.3 | 75.32 |
| 7rsa | 15909.9 | 16152.8 | 75.40 |
| 1aep | 19285 | 19593.3 | 76.17 |
| 1jpc | 13204.3 | 14075.5 | 76.34 |
| 1vls | 18689.3 | 19421.7 | 78.91 |
| 2aak | 20200.5 | 20330.8 | 79.75 |
| 1xjo | 33590.9 | 34157.4 | 79.97 |
| 1amm | 24208 | 25079.8 | 80.73 |
| 1mla | 39239.1 | 38549.4 | 81.55 |
| 1ad2 | 29637.1 | 29160.4 | 81.63 |
| 1nox | 27195.8 | 26599.2 | 81.64 |
| 1akz | 30738.2 | 30650.2 | 81.76 |
| 1xsm | 41236.8 | 40782.6 | 82.81 |
| 1ako | 37803.6 | 37354.7 | 82.97 |
| 1han | 37972.1 | 37900.1 | 83.41 |
| 1air | 44558.3 | 45452.7 | 83.56 |
| 1gnd | 61577.9 | 58899.4 | 85.72 |
| 1aa6 | 99503.2 | 94252.3 | 86.38 |
| 1alo | 120846.1 | 118421.6 | 86.98 |
| 1kit | 103772.6 | 101172.2 | 87.26 |
| 8catA | 70353.4 | 68895.4 | 86.98 |
| 1kit | 103772.6 | 101172.2 | 87.27 |
| 1gpb | 120845.6 | 115900.9 | 87.40 |
| 1qba | 125154.4 | 116908.8 | 87.48 |
| 1oacA | 102370.8 | 97918 | 87.59 |
| 2cas | 75066.7 | 74830.9 | 87.65 |
| 1bglA | 147042.7 | 141837.9 | 88.13 |

# References


[1] N. J. Higham, Functions of Matrices: Theory and Computation, SIAM, Philadelphia, PA, 2008.

[2] C. B. Moler and C. F. Van Loan, Nineteen dubious ways to compute the exponential of a matrix, SIAM Rev. 20 (1978) pp. 801–836.

[3] C. B. Moler and C. F. Van Loan, Nineteen dubious ways to compute the exponential of a matrix, twenty-five years later, SIAM Rev. 45 (2003) pp. 3–49.

[4] N. J. Higham, The scaling and squaring method for the matrix exponential revisited. SIAM J. Matrix Anal. Appl. 26 (2005) pp. 1179-1193.

[5] N. J. Higham, The scaling and squaring method for the matrix exponential revisited. SIAM Rev. 51 (2009) 747-764.

[6] M. Benzi, and C. Klymko, Total communicability as a centrality measure, J. Complex Net. 1 (2013) pp. 124-149.

[7] M. Benzi and P. Boito, Quadrature rule-based bounds for functions of adjacency matrices. Lin. Algebra Appl. 433 (2010) pp. 637-652.

[8] R. Milo, S. Shen–Orr, S. Itzkovitz, N. Kashtan, D. Chklovskii, and U. Alon Network motifs: simple building blocks of complex networks, Science, vol. 298 no. 5594 (2002), pp. 824–827.

[9] Myers, Christopher R. Software systems as complex networks: Structure, function, and evolvability of software collaboration graphs. Physical Review E 68 (2003): 046116.

[10] Berman, Helen M., John Westbrook, Zukang Feng, Gary Gilliland, T. N. Bhat, Helge Weissig, Ilya N. Shindyalov, and Philip E. Bourne. The protein data bank. Nucleic acids research 28, (2000): 235-242.

[11] Atilgan, Ali Rana, Pelin Akan, and Canan Baysal. Small-world communication of residues and significance for protein dynamics. Biophysical journal 86.1 (2004): 85-91.

[12] Fleming, Patrick J., and Frederic M. Richards. Protein packing: dependence on protein size, secondary structure and amino acid composition. Journal of molecular biology 299.2 (2000): 487-498.

[13] Voss, Neil R., and Mark Gerstein. 3V: cavity, channel and cleft volume calculator and extractor. Nucleic acids research (2010): gkq395.

[14] Lockwood, J. L., Powell, R. D., Nott, M. P., & Pimm, S. L. (1997). Assembling ecological communities in time and space. Oikos, 549-553.

[15] Rossberg, A. G., Matsuda, H., Amemiya, T., & Itoh, K. (2006). Food webs: experts consuming families of experts. Journal of Theoretical Biology, 241(3), 552-563.

[16] Estrada, E.; Hatano, N., Statistical-mechanical approach to subgraph centrality in complex networks. Chemical Physics Letters 439, 2007, 247-251.

[17] Sporns, Olaf, and Rolf Kötter. Motifs in brain networks. PLoS biology 2, no. 11 (2004): e369.

[18] Yodzis, P. (2000). Diffuse effects in food webs. Ecology 81, 261-266.

[19] Polis, G. A. (1991). Complex trophic interactions in deserts: an empirical critique of food-web theory. Am. Nat. 138, 123-155.

[20] Townsend, C., Thompson, R. M., McIntosh, A. R., Kilroy, C., Edwards, E., and Scarsbrook, M. R. (1998). Disturbance, resource supply, and food-web architecture in streams. Ecol. Lett. 1, 200.

[21] Christian, R. R., and Luczkovich, J. J. (1999). Organizing and understanding a winter's seagrass foodweb network through effective trophic levels. Ecol. Model. 117, 99-124

[22] Warren, P. H. (1989). Spatial and temporal variation in the structure of a fresh-water food web. Oikos 55, 299-311.

[23] Waide, R. B., and Reagan, W. B. (Eds.) (1996). The Food Web of a Tropical Rainforest. University Chicago Press, Chicago.

[24] N. D. Martinez, B. A. Hawkins, H. A. Dawah, and B. P. Feifarek, Effects of sampling efforts on characterization of food web structure, Ecology 80 (1999), pp. 1044–1055.

[25] Havens, K. (1992). Scale and structure in natural food webs. Science 257, 1107-1109.

[26] Opitz, S. (1996). Trophic Interactions in Caribbean coral reefs. ICLARM Tech. Rep. 43, Manila, Philippines, 341 pp.

[27] Memmott, J., Martinez, N. D., and Cohen, J. E. (2000). Predators, parasites and pathogens: species richness, trophic generality, and body sizes in a natural food web. J. Animal Ecol. 69, 1-15.

[28] Link, J. (2002). Does food web theory work for marine ecosystems? Mar. Ecol. Prog. Ser. 230, 1-9.

[29] Yodzis, P. (1998). Local trophodynamics and the interaction of marine mammals and fisheries in the Benguela ecosystem. J. Anim. Ecol. 67, 635-658.

[30] Goldwasser, L., and Roughgarden, J. A. (1993). Construction and analysis of a large Caribbean food web. Ecology 74, 1216-1233.

[31] Martinez, N. D. (1991). Artifacts or attributes? Effects of resolution on the Little Rock Lake food web. Ecol. Monogr. 61, 367-392.

[32] Baird, D., and Ulanowicz, R. E. (1989). The seasonal dynamics of the. Chesapeake Bay ecosystem. Ecol. Mon. 59, 329-364.

[33] Huxman, M., Beany, S., and Raffaelli, D. (1996). Do parasites reduce the chances of triangulation in a real food web? Oikos 76, 284-300.

[34] Hall, S. J., and Rafaelli, D. (1991). Food-web patterns - lessons from a species-rich web. J. Anim. Ecol. 60, 823–842.

[35] Hummon, N. P., Doreian, P., and Freeman, L. C. (1990). Analyzing the structure of the centrality-productivity literature created between 1948 and 1979. Know.-Creat. Diffus. Util. 11, 459-480.

[36] de Nooy, W., Mrvar, A., and Batagelj, V. (2005). Exploratory Social Network Analysis with Pajek, Cambridge University Press, Cambridge.

[37] Batagelj, V., and Mrvar, A. (2001). Graph Drawing Contest 2001. http://vlado.fmf.uni-lj.si/pub/GD/GD01.htm.

[38] ODLIS (2002). Online Dictionary of Library and Information Science http://vax.wcsu.edu/library/odlis.html.

[39] Roget´s Thesaurus of English Words and Phrases (2002). Project Gutenberg. http://gutenberg.net/etext/22.

[40] Batagelj, V., and Mrvar, A. (2006). Pajek datasets. Available at: http://vlado.fmf.uni-lj.si/pub/networks/data/.

[41] Uetz, P., Dong, Y.-A., Zeretzke, Ch., Atzler, C., Baiker, A., Berger, B., Rajagopala, S. V., Roupelieva, M., Rose, D., Fossum, E., and Haas, J., (2006). Herpesviral protein networks and their interaction with the human proteome, Science 311, 239-242.

[42] LaCount, D., Vignali, M., Chettier, R., Phansalkar, A., Bell, R., Hesselberth, J., Schoenfeld, L., Ota, I., Sahasrabudhe, S., Kurschner, C., Fields, S., Hughes, R. (2005). A protein interaction network of the malaria parasite Plasmodium falciparum. Nature 438, 103–107.

[43] Rual, J.-F., Venkatesan, K., Hao, T., Hirozane-kishikawa, T., Dricot, A., Ning, L., Berriz, G. F.,Gibbons, F. D., Dreze, M., Ayivi-Guedehoussou, N., Klitgord, N., Simon, C., Boxem, M., Milstein, Stuart., Rosenberg, J., Goldberg, D. S., Zhang, L. V., Wong, S. L., Franklin, G., Li, S., Albala, J. S., Lim, J., Fraughton, C., Llamosas, E., Cevik, S., Bex, C., Lamesch, P., Sikorski. R. S., Vandenhaute, J.,Zoghbi, H. Y., Smolyar, A., Bosak, S., Sequerra, R., Doucette-Stamm, L.,Cusick, M. E., Hill, D. E., Roth, F. P., and Vidal, M., (2005). Towards a proteome-scale map of the human protein-protein interaction network, Nature 437, 1173-1178.

[44] Bu, D., Zhao, Y., Cai, L., Xue, H., Zhu, X., Lu, H., Zhang, J., Sun, S., Ling, L., Zhang, N., Li, G., and Chen, R., (2003). Topological structure analysis of the protein-protein interaction network in budding yeast, Nucleic Acids Res. 31, 2443-2450.

[45] von Mering, C., Krause, R., Snel, B., Cornell, M., Oliver, S. G., Fields, S., and Bork, P., (2002). Comparative assessment of large-scale data sets of protein-protein interactions, Nature 417, 399-403.

[46] Motz, M., Kober, I., Girardot, C., Loeser, E., Bauer, U., Albers, M., Moeckel, G., Minch, E., Voss, H., Kilger, C., and Koegl, M. (2002). Elucidation of an Archaeal Replication Protein Network to Generate Enhanced PCR Enzymes. J. Biol. Chem. 277, 16179–16188.

[47] Lin, C. Y., Chen C. L., Cho, C. S., Wang L. M., Chang C. M., Chen P. Y., Lo, C. Z., and Hsiung, C. A. (2005). hp-DPI: Helicobacter pylori database of protein interactomes, A combined experimental and inferring interactions. Bioinformatics 21, 1288–1290.

[48] Davidson, E. H., Rast, J. P. Oliveri, P. Ransick, A., Calestani, C., Yuh, C. H., Minokawa, T., Amore, G., Hinman, V., Arenas-Mena, C., Otim, O., Brown, C. T., Livi, C. B., Lee, P. Y., Revilla, R., Rust, A. G., Pan, Z., Schilstra, M. J., Clarke, P. J., Arnone, M. I., Rowen, L., Cameron, R. A., McClay, D. R., Hood, L., and Bolouri, H. (2002). A genomic regulatory network for development. Science, 295, 1669 – 1678.

[49] Bultland, G., Peregrín-Alvarez, J. M., Li, J., Yang, W., Yang, X., Canadien, V., Starostine, A., Richards, D., Beattie, B., Krogan, N., Davey, M., Parkinson, J., Greenblatt, J., and Emili, A., (2005). Interaction network containing conserved and essential protein complexes in Escherichia coli, Nature, 433, 531-537.

[50] Noirot, P., and Noirot-Gross, N. F. (2004). Protein interaction networks in bacteria. Curr. Op. Microb. 7, 505–512.

[51] Milo, R., Itzkovitz, S., Kashtan, N., Levitt, R., Shen-Orr, Shai., Ayzenshtat, I., Sheffer, M.,and Alon, U., (2004a). Superfamilies of evolved and designed Networks, Science 303, 1538-1542.

[52] Shen-Orr, S. S., Milo, R., Mangan, S., and Alon, U. (2002). Network motifs in the transcriptional regulation network of Escherichia coli, Nature Gen. 31, 64-68.

[53] Davis, G. F., Yoo, M., and Baker, W. E. (2003). The Small World of the American Corporate Elite, 1982-2001. Strategic Organization 1, 301-326.

[54] MacRae, D. (1960). Direct factor analysis of sociometric data. Sociometry 23, 360-371.

[55] Lusseau, D., (2003). The emergent properties of a dolphin social network, Proc. R. Soc. Lond. B (Suppl.) 270, 186-188.

[56] Moody, J. (2001). Data for this project was provided in part by NIH grants DA12831 and HD41877, those interested in obtaining a copy of these data should contact James Moody (moody.77@sociology.osu.edu).

[57] Zachary, W. (1977).An information flow model for conflict and fission in small groups. J. Anthropol. Res. 33, 452-473.

[58] Zeleny, L. D. (1950). Adaptation of research findings in social leadership to college classroom procedures. Sociometry 13, 314-328.

[59] Potterat, J. J., Philips-Plummer, L., Muth, S. Q., Rothenberg, R. B., Woodhouse, D. E., Maldonado-Long, T. S., Zimmerman, H. P., Muth, J. B. (2002). Risk network structure in the early epidemic phase of HIV transmission in Colorado Springs. Sex. Transm. Infect. 78, i159-i163.

[60] Krackhardt, D. (1999). The ties that torture: Simmelian tie analysis in organizations. Res. Sociol. Org. 16, 183-210.

[61] Michael, J. H., and Massey, J. G. (1997). Modeling the communication network in a sawmill. Forest Prod. J. 47, 25-30.

[62] Faloutsos, M., Faloutsos, P., and Faloutsos, C. (1999). On power-law relationships of the internet topology. Comp. Comm. Rev. 29, 251-262.

[63] Watts, D.J., Strogatz, S.H., 1998. Collective dynamics of small-world networks. Nature 393, 440-442.

[64] Hanna, S.; (2009) Spectral comparison of large urban graphs. In: Koch, D. and Marcus, L. and Steen, J., (eds.) Proceedings of the 7th International Space Syntax Symposium. (pp. p. 39). Royal Institute of Technology (KTH): Stockholm, Sweden.

[65] Perna, A., Valverde, S., Gautrais, J., Jost, C., Solé, R. V., Kuntz, P., and Theraulaz, G. (2008). Topological efficiency in the three-dimensional gallery networks of termite nests. Physica A 387, 6235-6244.

[66] Buhl, J., Gautrais, J., Solé, R. V., Kuntz, P., Valverde, S., Deneubourg, J. L., and Theraulaz, G. (2004). Efficiency and robustness in ant networks of galleries. Eur. Phys. J. B 42, 123-129.
